# Supplementary material for: Non-perturbative improvement of the axial current with three dynamical flavors and the Iwasaki gauge action
Source: arXiv:hep-lat/0703006 source file (2007-03-12)
Supplement: Supplementary file 1 [file 7.appendix.tex]

\clearpage 

\appendix

\section{Results from a test run in two-flavor QCD}

\bi
   \item Here I list results from a test run in two-flavor QCD 
         at $\beta\!=\!2.0$.
   \item These are difficult to include in the paper, 
         since there is no measurement of $r_0$...
\ei

\begin{table}[htbp]
\begin{center}
\begin{tabular}{lllllllll}
   \hline
   $\beta$ & $L/a$ & $\kappa$ & $N_{\rm MD}$  & HMC traj. 
                         & $P_{\rm HMC}$ \\
   \hline
   2.00 & 12 & 0.13660 &  80 & 4000 & 0.86 \\ 
   2.00 & 12 & 0.13687 & 100 & 4000 & 0.89 \\ 
   2.00 & 12 & 0.13716 & 100 & 4000 & 0.87 \\ 
   \hline
\end{tabular}       
\caption{
   Simulation parameters. 
}
\label{tbl:nf2:simparam}
\end{center}
\end{table}

\begin{table}[htbp]
\begin{center}
\begin{tabular}{lll}
   \hline
   $\kappa$     & $am$       & $\cA$       \\ 
   \hline
   0.13660 &  0.01604(51) & -0.0561(27) \\
   0.13687 &  0.00772(54) & -0.0479(42) \\
   0.13716 & -0.00293(64) & -0.0465(33) \\
   \hline
\end{tabular}
\caption{
   Numerical results for $am$ and $\cA$ in two-flavor QCD 
   at $\beta\!=\!2.0$.
}
\label{tbl:nf2:cA:sim_mq}
\end{center}
\end{table}

\vspace{5mm}
\begin{figure}[htbp]
\begin{center}
   \includegraphics[width=80mm,clip]{Fig/cA_vs_mq_nf2.eps}
   \caption{
      Non-perturbative estimate of $\cA$ in two-flavor QCD at $\beta\!=\!2.0$
      as a function of $m$.
   }
   \label{fig:nf2:cA_vs_mq}
\end{center}
\end{figure}
